# Supplementary material for: Polarization switching mechanism in HfO$_2$ from first-principles lattice mode analysis
Source: arXiv:2108.12538 ancillary file (2021-08-28)
Supplement: Supplementary file 1 [file Supplementary_Materials.pdf]

# Supplementary Materials: Polarization switching mechanism in $HfO_2$ from first-principles lattice mode analysis

Yubo Qi, Sobhit Singh, and Karin M. Rabe
*Department of Physics & Astronomy, Rutgers University, Piscataway, New Jersey 08854, United States*

## I. POLYMORPHS IN $HFO_2$

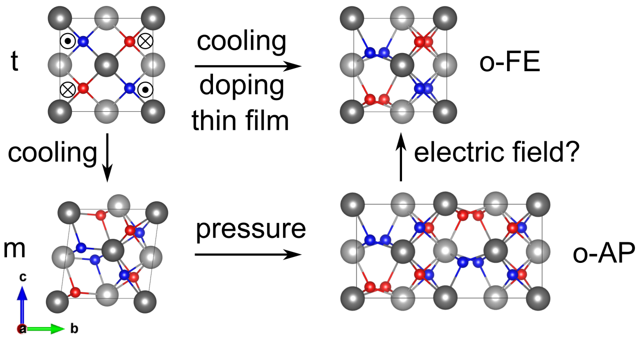


FIG. S1. Structures and transitions of various $HfO_2$ phases. The dark and light grey spheres represent closer and farther Hf atoms respectively. The blue and red colors indicate the oxygen atoms that are outward and inward displaced.

In Fig. S1, we show the schematic plot illustrating the phase transition between different $HfO_2$ phases. At high temperatures ($T >$ 2900 K), bulk $HfO_2$ has a cubic fluorite structure with space group $Fm\bar{3}m$ [S1]. As the temperature decreases (2900 K> $T$ >2073 K), this cubic structure transforms to a tetragonal $P4_2/nmc$ (denoted as t) phase [S1]. Upon further cooling ($T <$ 2073 K), bulk $HfO_2$ transforms to its ground state $P2_1/c$ monoclinic phase [S1]. The t phase can be induced to transform to the o-FE phase through specific techniques, such as doping, growth in thin film form, quenching, or imposing mechanical confinement, during cooling. Further, applying hydrostatic pressure to the ground state monoclinic phase can induce a transformation to the orthorhombic $Pbca$ o-AP phase.

## II. METHODS

Density-functional theory (DFT) calculations are carried out with the ABINIT package for structure optimizations of bulk $HfO_2$ with fixed lattice modes and the Quantum–espresso package for the nudged elastic band (NEB) calculations [S2]. The exchange-correlation functional is approximated with the local density approximation (LDA). The norm-conserving pseudopotentials are generated by the Opium package. The atomic force convergence threshold is set as $2\times10^{-4}$ Hartree per Bohr. A 4×4×4 Monkhorst–Pack $k$-point mesh is used to sample the Brillouin zone [S3]. The structure optimizations with fixed lattice modes are performed with the 'wtatcon' command in the ABINIT package.

The results we have presented in this work are based on calculations with the LDA functional. We note that both LDA and GGA functionals have been used in previous studies of $HfO_2$ based materials [S4–S8]. Using the generalized gradient approximation (GGA) changes the relative energy of each phase, but rarely destabilizes any of the phases. Our calculations show that the t phase is also a metastable phase in GGA calculations. The comparison between the lattice constants and energies given by LDA and GGA calculations is shown in Table S1, showing that the energy difference between the t phase and the o-FE phase is larger in GGA calculations. In Figure S2, we show the minimum energy paths during the two categories of uniform polarization switching given by LDA and GGA. We observe that the t phase is the intermediate state(s) no matter whether the functional is LDA or GGA, indicating that using the GGA functional does not influence the underlying physics about polarization switching presented in this work.

| functional | phase | $a$ | $b$ | $c$ | $E_1$ (eV) | $E_2$ (eV) |
|---|---|---|---|---|---|---|
| LDA | t | 4.93 | 4.89 | 4.89 | 0.121 | 0.205 |
| | o-FE | 5.07 | 4.87 | 4.88 | 0 | 0 |
| GGA | t | 5.20 | 5.04 | 5.04 | 0.304 | 0.312 |
| | o-FE | 5.24 | 5.01 | 5.05 | 0 | 0 |

TABLE S1. Comparison between LDA and GGA results in lattice parameters and relative energies of the t and o-FE phases. The energy of the o-FE phase is taken as the zero. $E_1$ is the energy given by a variable-cell calculation. $E_2$ is the energy of the structure whose lattice parameters are fixed as the ones of the o-FE phase. All length and energy units are in Åand eV/cell respectively.

## III. SYMMETRY-ADAPTED LATTICE MODES

### A. Schematic Illustration of Lattice Modes

In Fig. S3, we show the schematic illustrations of the oxygen displacements in different lattice modes.

In Fig. S4, we demonstrate how these lattice modes are reflected in the o-FE structure. The o-FE phase is composed of a polar three-fold oxygen layer and a non-polar four-fold oxygen layer, which result form a constructive interference and destructive interference of the $\Gamma_{15}^{Z}$ and

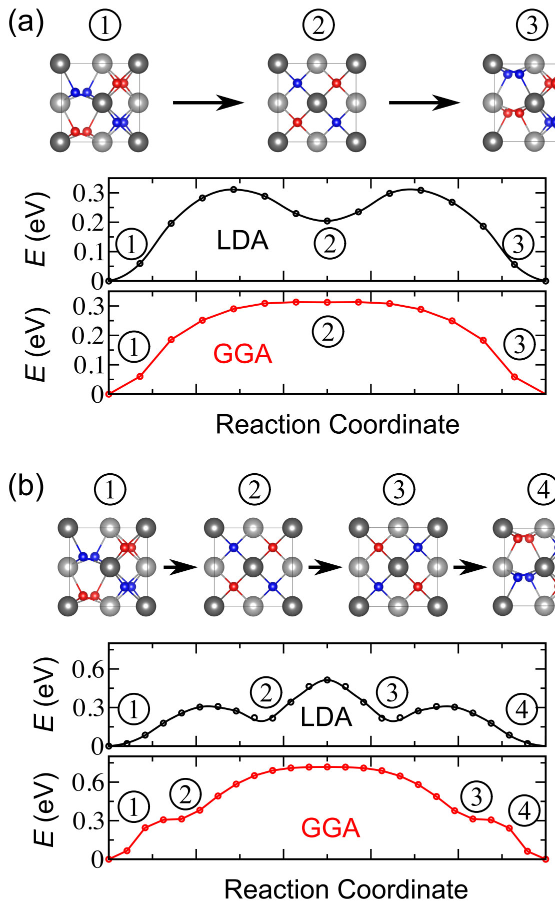


FIG. S2. Comparison between the LDA and GGA results about the minimum energy paths during the two categories of uniform polarization switching.

$Y_5^Z$ modes respectively, as shown in Fig. S4 (a). The magnitudes of the $x$-direction displacements are different in the three-fold and four-fold oxygen layers (indicated by the dashed circles). The four-fold oxygen atoms have small displacements, indicated by the pale red and blue colors. This is a result of the constructive interference and destructive interference of the $X_2^-$ and $Z_5^X$ modes [Fig. S4 (b)]. Fig. S4 (c) shows the character of the $X_5^Y$ mode. Viewing along the $x$-direction, the oxygen atoms, which overlap in the high-symmetry cubic structure, separates along the $y$-direction

### B. Different variants of down-polarized structures

In Table S2, we show the amplitudes of lattice modes in different variants of the down polarized states. In Fig. S5, we show the comparison between the up-polarized structure and different variants of the down polarized states.

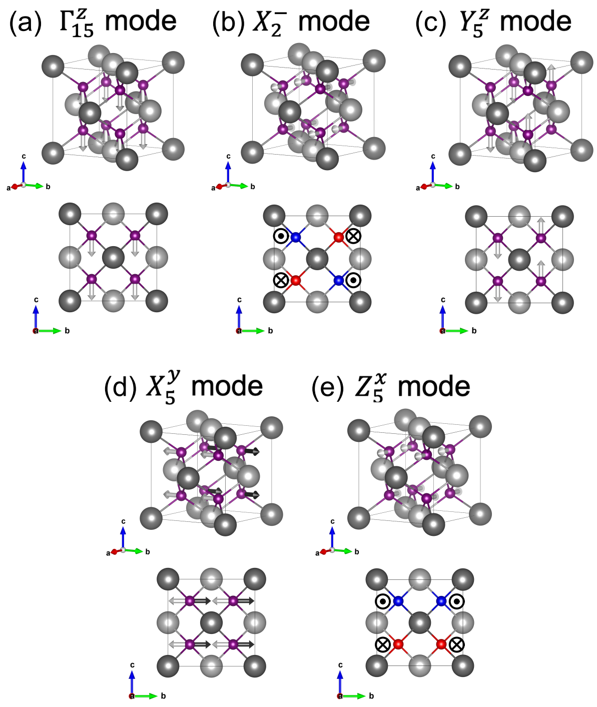


FIG. S3. Schematic illustrations of the oxygen displacements in the lattice modes $X_2^-$, $\Gamma_{15}^Z$, $Y_5^Z$, $X_5^Y$, and $Z_5^X$ respectively.

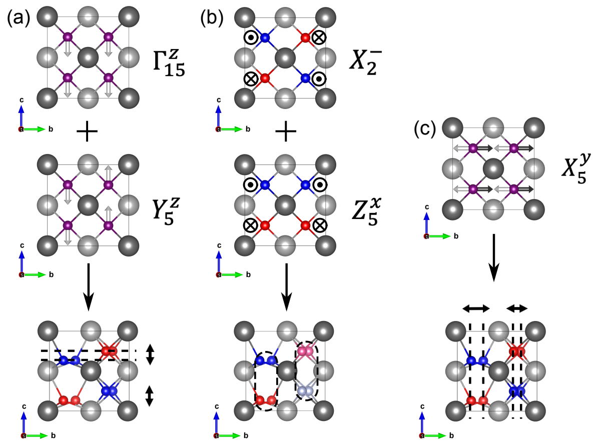


FIG. S4. Schematic figures illustrating how different lattice modes are reflected in the o-FE structure. In this figure, in order to highlight that the 3-fold and 4-fold oxygen atoms have different magnitudes of $x$-direction displacements, the 4-fold oxygen atoms are colored with pale red and pale blue. In the other part of this paper, we color all oxygen atoms with red and blue only according to the directions of displacements, since the magnitudes are not important.

### C. Coupling between Lattice Modes

In Fig. S6, we show how the anti-polar modes couple with the polar $\Gamma_{15}^Z$ mode. We begin with the o-FE structure, artificially decrease the $Q\left(\Gamma_{15}^Z\right)$ gradually.

| | $\Gamma_{15}^z$ | $X_2'$ | $X_5^Y$ | $Y_5^Z$ | $Z_5^X$ | Operation |
|---|---|---|---|---|---|---|
| Up-polarized | 0.238 | 0.473 | 0.409 | 0.402 | 0.394 | |
| type I | -0.238 | 0.473 | -0.409 | -0.402 | 0.394 | $\sigma_y\sigma_z$ |
| type II | -0.238 | 0.473 | -0.409 | 0.402 | -0.394 | $\sigma_x\sigma_z$ |
| type III | -0.238 | -0.473 | 0.409 | 0.402 | 0.394 | $\sigma_x\sigma_y\sigma_z$ |
| type IV | -0.238 | -0.473 | 0.409 | -0.402 | -0.394 | $\sigma_z$ |

TABLE S2. Amplitudes of the lattice modes in the four different down-polarized variants.

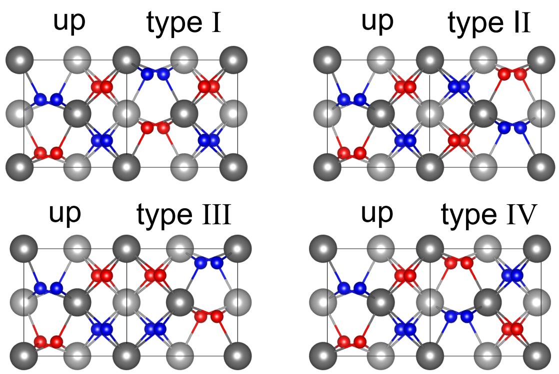


FIG. S5. Comparisons between the up-polarized structure and four different down-polarized variants. An up-polarized structure is placed adjacent to the four different down-polarized variants respectively, forming an non-optimized 180° domain structure.

At each step, we optimize the structure with $Q\left(\Gamma_{15}^Z\right)$ fixed, and the changes of the amplitudes of the anti-polar modes with respect to $Q\left(\Gamma_{15}^Z\right)$ is shown in Fig. S5. At $Q\left(\Gamma_{15}^Z\right) = 0.108$ Å, the o-FE phase becomes unstable and transforms to the structure with the *Aba*2 space group. This first-order phase transition is associated with jumps in the amplitudes of all the anti-polar modes. To investigate the (meta)stability of the *Aba*2 around the critical mode amplitude, we start with the *Aba*2 phase, increase the $Q\left(\Gamma_{15}^Z\right)$ gradually (these data are represented by open circles linked by a dashed line). As shown in the zoomed figure (Fig. S5 (a)), the *Aba*2 phase becomes unstable at $Q\left(\Gamma_{15}^Z\right) = 0.118$ Å.

### D. Energetic Terms

The terms appear in a Landau-type energetic expression should be invariant upon operations. To figure out the allowed lowest-order terms, we consider operations including 2-fold rotations, mirror reflections, and inversions. The sign up to which each mode transforms into itself under a specific operation is summarized in Table S3. From the table, we can see that terms $a_1Q\left(X_2^-\right)^2$, $a_2Q\left(\Gamma_{15}^Z\right)^2 Q\left(X_2^-\right)^2$, $a_3Q\left(X_2^-\right)Q\left(\Gamma_{15}^Z\right)Q\left(X_5^Y\right)$, and $a_4Q\left(X_2^-\right)Q\left(\Gamma_{15}^Z\right)Q\left(Y_5^Z\right)Q\left(Z_5^X\right)$ are invariant upon these operations and thus allowed in a Landau-type en-

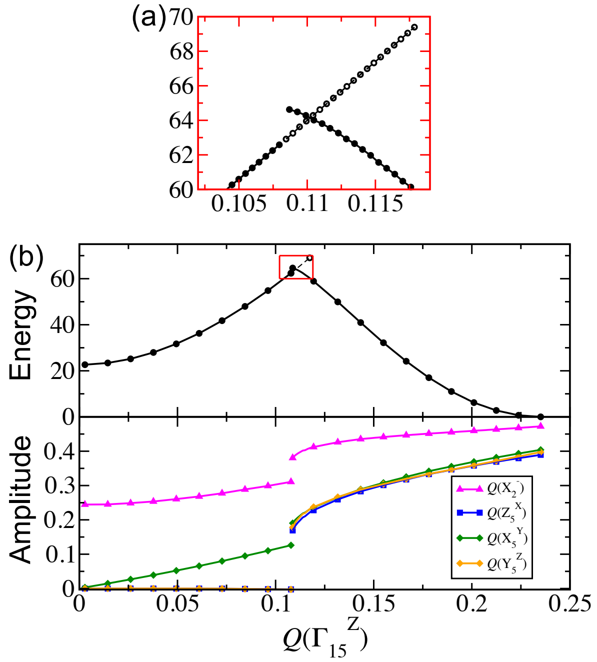


FIG. S6. The changes of the amplitudes of anti-polar modes $X_2^-$, $Y_5^Z$, $X_5^Y$, and $Z_5^X$ with respect to $Q\left(\Gamma_{15}^Z\right)$.

ergetic expression.

| | $C_x^2$ | $C_y^2$ | $C_z^2$ | $\sigma_x$ | $\sigma_y$ | $\sigma_z$ | $I$ |
|---|---|---|---|---|---|---|---|
| $\Gamma_{15}^Z$ | -1 | -1 | 1 | 1 | 1 | -1 | -1 |
| $X_2^-$ | 1 | 1 | 1 | -1 | -1 | -1 | -1 |
| $X_5^Y$ | -1 | -1 | 1 | -1 | -1 | 1 | 1 |
| $Y_5^Z$ | 1 | -1 | -1 | 1 | -1 | -1 | 1 |
| $Z_5^X$ | -1 | 1 | -1 | -1 | 1 | -1 | 1 |

TABLE S3. Table summarizing the sign up to which each mode transforms into itself under a specific operation.

## IV. SUPPLEMENTARY PART OF FIG. 3

Fig. S7 is the supplementary part of Fig. 3 in the main text. Fig. 3 shows the energy profiles and mode-amplitude evolutions during the structural changes toward the type I and type III down-polarized states. And Fig. S7 shows the energy profiles and mode-amplitude evolutions during the structural changes toward the type II and type IV down-polarized states. The energy profiles, changes of the $\Gamma_{15}^Z$, $X_2^-$, and $X_5^Y$ modes are identical during first category switching, in which that final states are the type I and type II down-polarized states. During the flipping to the type I down-polarized state, after passing the intermediate state, $Q\left(Y_5^Z\right)$ becomes positive and $Q\left(Z_5^X\right)$ becomes negative. However, during the

flipping to the type II down-polarized state, after passing the intermediate state, $Q\left(Y_5^Z\right)$ becomes negative and $Q\left(Z_5^X\right)$ becomes positive. Similarly, the energy profiles, changes of the $\Gamma_{15}^Z$, $X_2^-$, and $X_5^Y$ modes are also identical during second category switching, in which that final states are the type III and type IV down-polarized states. During the flipping to the type III down-polarized state, after passing the second intermediate state, both $Q\left(Y_5^Z\right)$ and $Q\left(Z_5^X\right)$ becomes positive. However, during the flipping to the type IV down-polarized state, after passing the second intermediate state, both $Q\left(Y_5^Z\right)$ and $Q\left(Z_5^X\right)$ becomes negative. It is worth mentioning that these is another structural transformation path for the switching to the type IV down-polarized state. However, it has a large activation energy and cannot be the optimal path, which is discussed in this supplementary materials section VIII.

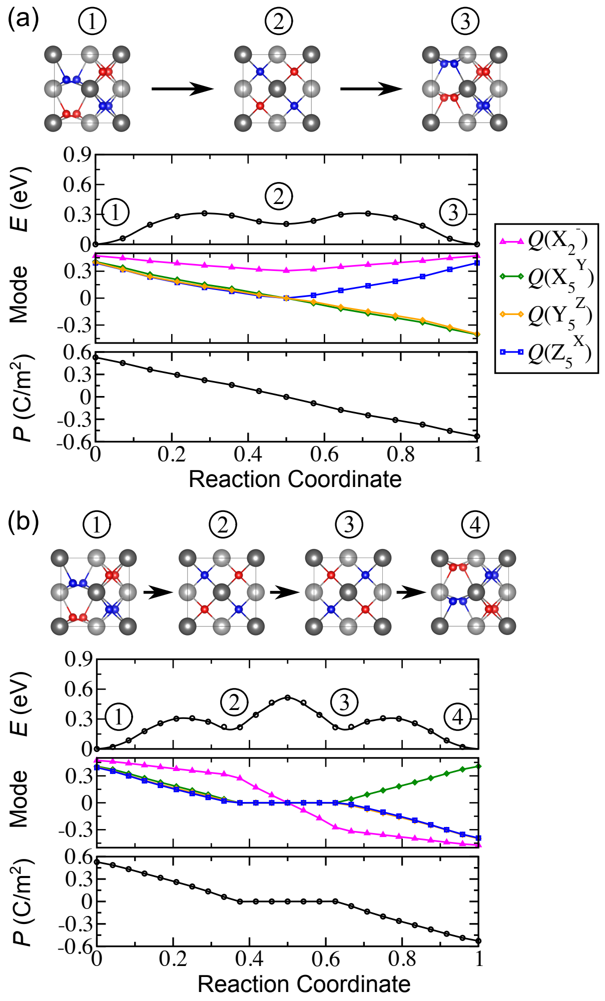


FIG. S7. Energy profiles and changes of lattice-mode amplitudes during the structural changes toward the type II and type IV down-polarized states.

## V. DOMAIN WALL ENERGIES

Our calculations show that the domain wall energies of the types I, II and III domain structures are much higher than the IV domain structure. This can be understood from the lattice mode arrangements. It is well known that the $HfO_2$ structures composed of 8-coordinated Hf atoms (such as the t and c phases) have higher energy than the structures composed of 7-coordinated Hf atoms (such as the o-FE and o-AP phases). As shown in Fig. S8 (a) and Fig. S6, in the type II and type III domain structures, the oxygen atoms attached to the Hf atoms at the domain wall have no displacements along the $z$ direction, indicating that the Hf atoms are 8-coordinated. On the other hand, the Hf atoms in the type IV domain structure (Fig. S8 (b)) are all 7-coordinated, indicating a lower energy. In the type I domain structure, the Hf atoms at the domain wall are 7-coordinated. However, different from the type IV domain structures (Fig. S8 (d)), the signs of the $X_5^Y$ mode are opposite across the domain wall (Table S3). As shown in Fig. S8 (c), this specific distortion pattern makes the oxygen atoms at the domain wall close to each other, leading to a larger Coulombic repulsion energy.

The energies of the first category domain wall structures are higher than that of the type IV domain wall structure. However, it does not mean that the first category domain wall structures are unlikely to form. The underlying reasons include but are not limited to the following two.

First, the energy barrier between the high temperature tetragonal phase and a first category domain wall structure is lower. Our calculations show that a tetragonal to type I domain structure requires 1.34 eV and a tetragonal to type IV domain structure requires 1.50 eV. If we anneal the crystal from a high temperature, it is possible that the structural transformation selects a path with lower energy barrier, rather than the one toward the lowest energy structure. Such a tetragonal to type I domain transformation is also in concert with the Ostwalds step rule [S9], which states that a phase transition may end with a phase with a closer free energy to that of the parent phase, rather than the phase with a lower energy.

Second, domain nucleation often begins from impurities, surfaces, and interfaces [S10, S11], where the domain wall formation energy is much lowered. Therefore, the physical quantity, which determines whether a domain wall propagation model is plausible, should be the domain wall motion energy, rather than formation energy.

## VI. TYPE I DOMAIN WALL PROPAGATION

In the type I domain wall propagation, the structure 2 in Fig. 4 (a), which has a tetragonal structure at the domain wall, has the lowest energy and is the most stable domain structure. Here, we calculate the activation energy for domain wall propagation starting from this

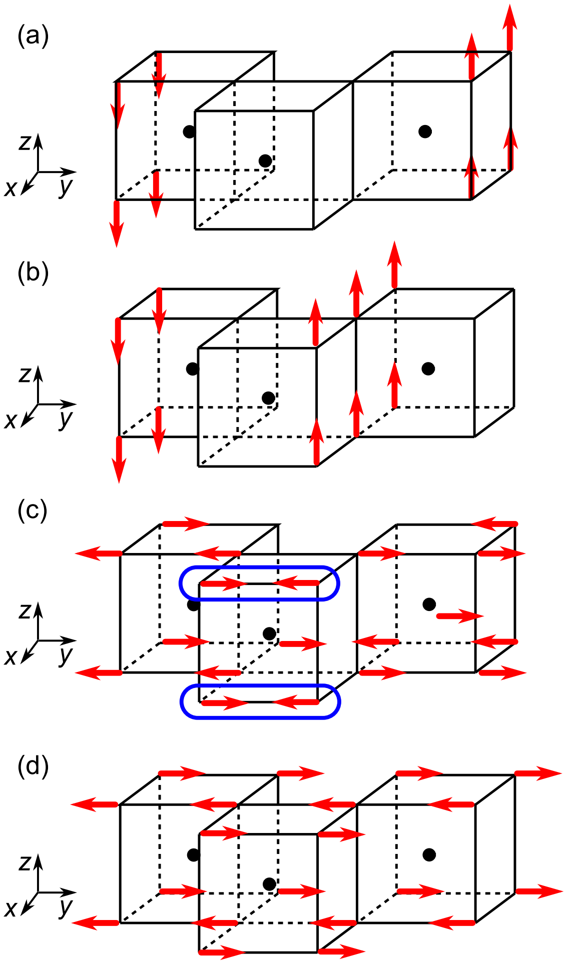


FIG. S8. (a) Schematic illustrations of the oxygen displacements along the $z$ direction in the type II and type III domain wall structure. The Hf atoms at the domain walls are 8-coordinated; (b) Oxygen displacements along the $z$ direction in the type I and type IV domain wall structure. The Hf atoms at the domain walls are 7-coordinated; (c) Oxygen displacements along the $y$ direction in the type I domain wall structure. The signs of $X_5^Y$ mode amplitudes in adjacent layers are opposite; (d) Oxygen displacements along the $y$ direction in the type IV domain wall structure. The signs of $X_5^Y$ mode amplitudes in adjacent layers are the same.

structure and expand the up-polarized domain by one unit cell. The initial structure is the structure 2 in Fig. 4 (a) and the intermediate state is the is the structure 3 in Fig. 4 (a). The energy profile is shown in Fig. S9.

## VII. FLIPPING A UNIT CELL IN THE O-AP PHASE

In Fig. S10 (a), we show the minimum energy paths for the transformation between the o-AP and o-FE phases (the black curve) and the switching the polarization of a unit cell in an 8-unit-cell o-AP supercell. The structures of the initial, transition, and final states are shown in

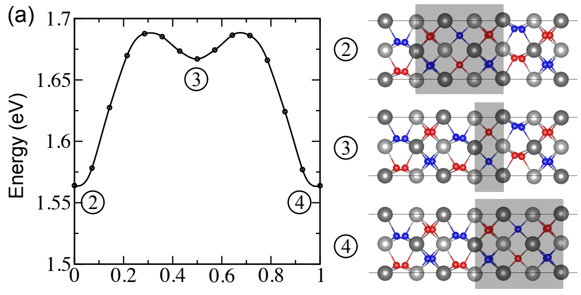


FIG. S9. Domain wall propagation starting from the most stable domain structure, which is the structure 2 in Fig. 4 (a) in the main draft.

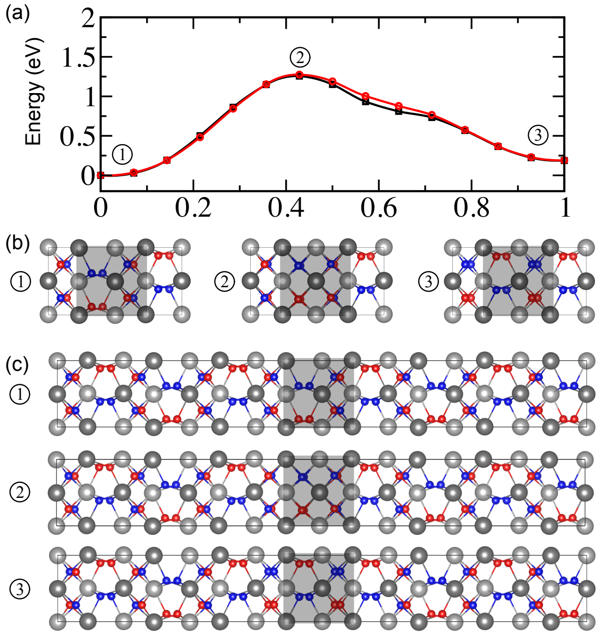


FIG. S10. The minimum energy paths for the transformation between the o-AP and o-FE phases (the black curve) and the switching the polarization of a unit cell in an 8-unit-cell o-AP supercell. The structures of the initial, transition, and final states are shown in (b) and (c). The unit cell whose polarization switches is shaded.

(b) and (c). We observe that the two energy profiles are approximately the same, further supporting that there is little interaction between domain wall. The energy barrier is 1.27 eV, which is much higher than the energy barriers in the first category domain wall propagations. Even thought transforming the o-AP phase (in which each up-polarized cell is neighbored with two type IV down polarized cells) into the o-FE phase is different from domain wall propagation (in which each up-polarized cell is neighbored with only one type IV down polarized cells) and uniform switching (in which each up-polarized cell is neighbored with zero type IV down polarized cells), they all require reversing $Q\left(X_2^-\right)$, which not only needs

a higher activation energy, but also can not be induced by an electric field.

## VIII. ANOTHER POLARIZATION SWITCHING PATH

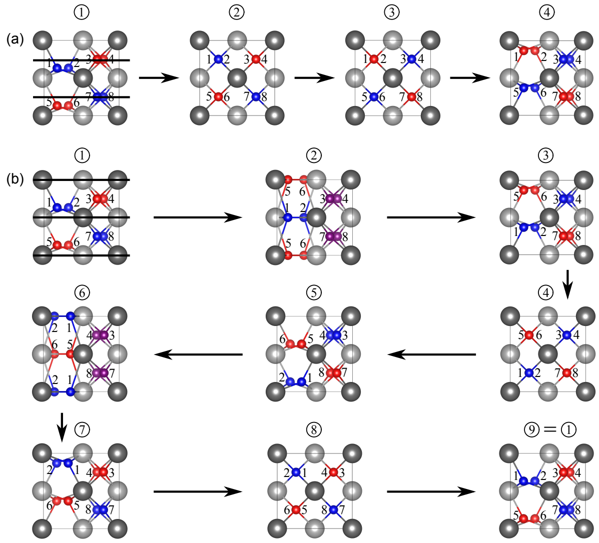

FIG. S11. The comparison between the two possible polarization switching paths connecting the up-polarized state and the type IV down-polarized state. (a) the polarization switching path in which the oxygen atoms move through the mid-planes (indicated by the solid lines) of the Hf planes. This path is also the one discussed in the main text. (b) structures 1-4 show another path, in which the oxygen atoms move through the planes (indicated by the solid lines) of the Hf planes. This path is not discussed in the main text, since the energy required to trigger the 1 to 4 structural transformation can make the system ionically conductive.

In Fig. S11, we show the comparison between the two possible polarization switching paths connecting the up-polarized state and the type IV down-polarized state. Subfigure (a) shows the path discussed in the main text. Subfigure (b) structures 1-4 show another path, which is not discussed in the main text. This is because the energy required to trigger the polarization switching in this path can make the system ionically conductive. In Table S4, we summarize the activation energy for the structural transformation in each step in subfigure (b). We see that the first step requires 0.73 eV, which is the highest. This means that if we apply an electric field which is big enough to transform structure 1 into structure 2, this field should be large enough to trigger all other transformations in subfigure (b). The structure 9 is the same as the structure 1, expect that the oxygen atoms 1,2,5 and 6 move by one unit cell. Under such an electric field, oxygen atoms 1,2,5 and 6 will keep moving, indicating that the system is ionically conductive.

[S1] J. Wang, H. P. Li, and R. Stevens, J. Mater. Sci. **27**, 5397 (1992).

[S2] P. Giannozzi, S. Baroni, N. Bonini, M. Calandra,

| | 1→2 | 2→3 | 3→4 | 4→5 | 5→6 | 6→7 | 7→8 | 8→9 |
|---|---|---|---|---|---|---|---|---|
| $E_a$ | 0.73 | 0.00 | 0.31 | 0.11 | 0.73 | 0.00 | 0.31 | 0.11 |

TABLE S4. Table summarizing the activation energy for each step in the path illustrated in Fig. S11 (b). The unit is eV.


R. Car, C. Cavazzoni, D. Ceresoli, G. L. Chiarotti, M. Cococcioni, I. Dabo, A. D. Corso, S. de Gironcoli, S. Fabris, G. Fratesi, R. Gebauer, U. Gerstmann, C. Gougoussis, A. Kokalj, M. Lazzeri, L. Martin-Samos, N. Marzari, F. Mauri, R. Mazzarello, S. Paolini, A. Pasquarello, L. Paulatto, C. Sbraccia, S. Scandolo, G. Sclauzero, A. P. Seitsonen, A. Smogunov, P. Umari, and R. M. Wentzcovitch, J. Phys.: Condens. Matter **21**, 395502 (2009).

[S3] H. J. Monkhorst and J. D. Pack, Phys. Rev. B **13**, 5188 (1976).

[S4] J. E. Jaffe, R. A. Bachorz, and M. Gutowski, Phys. Rev. B **72**, 144107 (2005).

[S5] X. Zhao and D. Vanderbilt, Phys. Rev. B **65**, 233106 (2002).

[S6] R. Materlik, C. Künneth, and A. Kersch, J. Appl. Phys. **117**, 134109 (2015).

[S7] T. D. Huan, V. Sharma, G. A. Rossetti Jr, and R. Ramprasad, Phys. Rev. B **90**, 064111 (2014).

[S8] K. Kamiya, N. Umezawa, and S. Okada, Phys. Rev. B **83**, 153413 (2011).

[S9] W. Z. Ostwald, Z. Phys. Chem **22**, 289 (1897).

[S10] C. T. Nelson, P. Gao, J. R. Jokisaari, C. Heikes, C. Adamo, A. Melville, S.-H. Baek, C. M. Folkman, B. Winchester, Y. Gu, Y. Liu, K. Zhang, E. Wang, J. Li, L.-Q. Chen, C.-B. Eom, D. G. Schlom, and X. Pan, Science **334**, 968 (2011).

[S11] S. G. Ingle, H. S. Dutta, and A. P. David, J. Appl. Phys. **64**, 4640 (1988).
